# Supplementary material for: Type Checking Program Code using SHACL (Extended Version)
Source: arXiv:1907.00855 source file (2019-07-01)
Supplement: Supplementary file 2 [file preservation.tex]

\documentclass{subfiles}
\begin{document}

\subsection{Proof of Preservation}

\begin{proof}
By induction of the derivation of $S,\Gamma \vdash t : T,S'$.
    \begin{description}
        \item[T-LET] 
            $t =\textbf{let}~x=t_1~\textbf{in}~t_2$,
            $S,\Gamma \vdash t_1 : T_1,S_1$,
            $S \cup S_1, (\Gamma, x:T_1) \vdash t_2 : T_2,S_2$.
            $S,\Gamma \vdash t : T_2,S_1 \cup S_2$,
            There are two ways $t$ can be reduced: E-LET and E-LETV.
            \begin{enumerate}
                \item $t' = \textbf{let}~x = t'_1~\textbf{in}~t_2$. By induction
                    hypothesis, $t_1 \rightarrow t'_1$ preserves the type. Then
                    by rule T-LET, $t' : T_2, S_1\cup S_2$. 
                \item $t' = \lbrack x \mapsto \mathit{val}_1 \rbrack t_2$. By
                    Lemma~\ref{lemma:substitution}, the type is preserved,
                    therefore $t' : T_2$. 
            \end{enumerate}

        \item[T-APP] 
            $t = t_1 t_2$,
            $S,\Gamma \vdash t_1 : T_{11} \rightarrow T_{12},S_1$,
            $S,\Gamma \vdash t_2 : T_{11}, S_2$,
            $S,\Gamma \vdash t_1 t_2 : T_{12}, S_1 \cup S_2$. 
            There are three rules by which $t'$ can be derived: E-APP1, E-APP2
            and E-APPABS. 
            \begin{enumerate}
                \item $t' = t_1' t_2$ By induction hypothesis, $t_1 \rightarrow
                    t'_1$ preserves the type. Therefore, by rule T-APP, $t'
                    : T_{12}$. 
                \item $t' = \mathit{val}_1 t'_2$. Same as first case. 
                \item $t' = \lbrack x \mapsto \mathit{val}_2 \rbrack t_{12}$. By
                    Lemma~\ref{lemma:substitution}, the type is preserved.
                    Therefore $t' : T_{12}$. 
            \end{enumerate}

        \item[T-IF]  
            $t = \textbf{if}~t_1~\textbf{then}~t_2~\textbf{else}~t_3$,
            $S,\Gamma \vdash t_1 : \text{bool}, S_1$,
            $S,\Gamma \vdash t : T_\mathit{lub}, S_1 \cup S_2 \cup S_3$.
            There are three rules by which $t'$ can be derived: E-IF, E-IF-TRUE
            and E-IF-FALSE. 
            \begin{enumerate}
                \item $t'=\textbf{if}~t'_1~\textbf{then}~t_2~\textbf{else}~t_3$.
                    By hypothesis, $t_1 \rightarrow t'_1$ preserves the type.
                    Therefore, by rule T-IF, $t : T_\mathit{lub}$.
                \item $t_1 = \text{true}$, $t' = t_2$. By the construction of
                    $T_\mathit{lub}$, it must be true that $t_2
                    <: T_\mathit{lub}$. Therefore, $t' : T_\mathit{lub}$.
                \item $t_1 = \text{false}$, $t' = t_3$. Same as second case. 
            \end{enumerate}

        \item[T-NIL] Vacuously fulfilled, since \textbf{nil} is a value.
        
        \item[T-CONS]
            $t = \textbf{cons}~t_1~t_2$,
            $S,\Gamma \vdash t_1 : T_1,S_1$,
            $S,\Gamma \vdash t_2 : T_1~\text{list},S_2$,
            $S, \Gamma \vdash t : T_1~\text{list},S_1 \cup S_2$. 
            There are two rules by which $t'$ can be derived: E-CONS1 and
            E-CONS2. 
            \begin{enumerate}
                \item $t' = \textbf{cons}~t'_1 t_2$. By hypothesis, $t_1
                    \rightarrow t'_1$ preserves the type. Therefore, by rule
                    T-CONS, $t' : T_1~\text{list}$. 
                \item $t' = \textbf{cons}~\mathit{val}_1 t'_2$. Same as first
                    case.
            \end{enumerate}

        \item[T-ABS] Vacuously fulfilled, since $\lambda (x:T).t_1$ is value. 
        \item[T-VAR] Cannot happen. 
        \item[T-TRUE] Vacuously fulfilled, since $\text{true}$ is a value. 
        \item[T-FALSE] Vacuously fulfilled, since $\text{false}$ is a value. 
        
        \item[T-NULL]
            $t = \textbf{null}~t_1$,
            $S, \Gamma \vdash t_1 : T_1~\text{list}, S_1$,
            $S, \Gamma \vdash t : \text{bool}, S_1$.
            There are three rules by which $t'$ can be derived: E-NULL,
            E-NULL-TRUE and E-NULL-FALSE. 
            \begin{description}
                \item $t' = \textbf{null}~t'_1$. By hypothesis, $t_1 \rightarrow
                    t'_1$ preserves the type. Therefore, by rule T-NULL, $t'
                    : \text{bool}$. 
                \item $t'_1 = \textbf{nil}$, $t' = \text{true}$. By rule T-TRUE,
                    $t' : \text{bool}$. 
                \item $t'_1 = \textbf{cons}~\mathit{val}_1 \ldots$, $t'
                    = \text{false}$. By rule T-FALSE, $t' : \text{bool}$. 
            \end{description}

        \item[T-HEAD]
            $t = \textbf{head}~t_1$,
            $S,\Gamma \vdash t_1 : T_1~\text{list}, S_1$. 
            $S, \Gamma \vdash t : T_1, S_1$. 
            There are two rules by which $t'$ can be derived: E-HEAD and
            E-HEADV. 
            \begin{enumerate}
                \item $t' = \textbf{head}~t'_1$. By hypothesis, $t_1 \rightarrow
                    t'_1$ preserves the type. Therefore, by rule T-HEAD, $t'
                    : T_1$. 
                \item $t_1 = \textbf{cons}~\mathit{val}_1 \ldots$, $t'
                    = \mathit{val}_1$. Due to rules T-CONS and T-HEAD,
                    $\mathit{val}_1$ must have type $T_1$. Therefore, $t'
                    : T_1$. 
            \end{enumerate}

        \item[T-TAIL]
            $t = \textbf{tail}~t_1$,
            $S,\Gamma \vdash t_1 : T_1~\text{list},S_1$,
            $S, \Gamma \vdash \textbf{tail}~t_1 : T_1~\text{list}, S_1$. 
            There are two rules by which $t'$ can be derived: E-TAIL and
            E-TAILV. 
            \begin{enumerate}
                \item $t' = \textbf{tail}~t'_1$. By hypothesis, $t_1 \rightarrow
                    t'_1$ preserves the type. Therefore, by rule T-TAIL, $t'
                    : T_1~\text{list}$.
                \item $t_1 = \textbf{cons}~\mathit{val}_1~\mathit{val}_2$, $t'
                    = \mathit{val}_2$. Due to rules T-CONS and T-TAIL,
                    $\mathit{val}_2$ must have type $T_1~\text{list}$,
                    Therefore, $t' : T_1~\text{list}$. 
            \end{enumerate}

        \item[T-RCD]
            $t = \{l_i=t_i^{i\in 1 \ldots n}\}$,
            $\text{for each } i~S,\Gamma \vdash t_i : T_i, S_i$,
            $S,\Gamma \vdash t : \{l_i : T_i^{i \in 1 \ldots n}\}, \bigcup_i=1^n
            S_i$.
            $t'$ can only be derived be rule E-RCD in which $t_i \rightarrow
            t'_i$. By hypothesis, this preserves the type.  
        
        \item[T-RCDPROJ]
            $t = t_1.l_j$,
            $S,\Gamma \vdash t_1 : \{l_i : T_i^{i\in 1 \ldots n}\}, S_1$,
            $S, \Gamma \vdash t : T_j, S_1$. 
            There are two rules by which $t'$ can be derived: E-PROJ and
            E-PROJRCD. 
            \begin{enumerate}
                \item $t' = t'_1.l_j$. By hypothesis, $t_1 \rightarrow t'_1$
                    preserves the type. Therefore, $t' : T_j$.
                \item $t = \{l_i = \mathit{val}_i^{i\in 1 \ldots n}\}$, $t'
                    = \mathit{val}_j$. Due to rule T-RCD and T-RCDPROJ,
                    $\mathit{val}_j$ must have type $T_j$. Therefore, $t'
                    : T_j$. 
            \end{enumerate}

        \item[T-QUERY] Immediate since rule E-QUERY applies. 

        \item[T-NPROJ]
            $t = t_1.l$,
            $S,\Gamma \vdash t_1 : s,S_1$.
            $S, \Gamma \vdash t : s'~\text{list}, S_1 \cup \{s',\geq_1 l^{-}.s,
            \emptyset\}$.
            There are two rules by which $t'$ can be derived: E-PROJ and
            E-PROJNODE. 
            \begin{enumerate}
                \item $t' = t'_1.l$. By hypothesis, $t_1 \rightarrow t'_1$
                    preserves the type. Therefore, $t' : s'$. 
                \item $t_1 = v$, $t'
                    = \textbf{cons}~\mu_1(x)~\ldots~\textbf{cons}~\mu_n(x)~\textbf{nil}$
                    with $\mu_i \in \llbracket l(v,x) \rrbracket_G$. Each node
                    $\mu_i(x)$ must fulfill the constraint $\geq_1 l^{-}.s$ of
                    shape $s'$ as it would otherwise not be in the query result.
                    Therefore, the type is preserved as $t' : s'~\text{list}$   
            \end{enumerate}

        \item[T-SUB] Results follows from induction hypothesis. 

\end{description}
\end{proof}

\end{document}
